# Supplementary material for: AutoURDF: Unsupervised Robot Modeling from Point Cloud Frames Using Cluster Registration
Source: arXiv:2412.05507 source file (2025-03-25)
Supplement: Supplementary file 1 [file X_suppl.tex]

\clearpage
\setcounter{page}{1}
\setcounter{section}{0}

 % This will use A, B, C for sections

\maketitlesupplementary
{\bf{Overview.}}
The supplementary material is structured into the following sections:
\begin{itemize}
\item Data Collection \ref{sec:data_collection}: This section describes the synthetic data generation process and real-world datasets used for evaluating the proposed method;
\item Method Details \ref{sec:method_details}: This section provides a detailed explanation of the topology inference algorithm, model architecture, and comparison between pose representations; 
\item Additional Experiments \ref{sec:additional_exp}: This section presents experiments analyzing the impact of varying frames, cameras, clusters, noise, and parameters, along with supplementary visualization results.
\end{itemize}

\section{Data Collection}
\label{sec:data_collection}

\subsection{Synthetic Data}
We simulate the robots and point cloud scanning process with Pybullet \cite{coumans2015bullet}.
The robot is controlled by randomly sampled motor angle sequences, and the corresponding point cloud frames are captured during this process. In the simulation, we collect 5 video sequences per robot, with each video containing 10 frames of point cloud data. To simulate real-world conditions, random positional noise and per-point noise are added to the point cloud data.
In the experimental results presented in the main text, we combine 20 camera views into a single frame point cloud to create dense point cloud. 
Figure \ref{fig_s1} illustrates the process of generating a single-frame point cloud from three views of depth images.

To ensure the point cloud sequence captures sufficient motion information, we independently sample random targets within the motor angle limits for each motor. Additionally, if the robot detects a self-collision, the sequence is restarted with a new set of target motor angles. Randomly sampled data may include similar rotational motions, making it challenging to identify distinct parts. Our method can merge multiple random motion sequences, improving the kinematics inference accuracy.
\begin{figure}[!t]
  \centering
  \begin{minipage}{\columnwidth}
    \centering
    \includegraphics[width=\columnwidth]{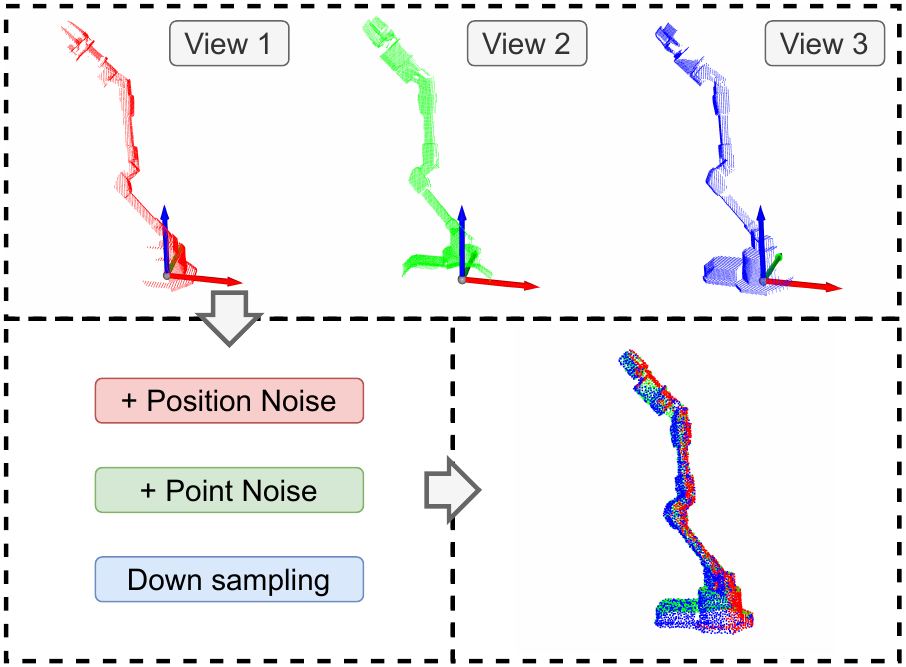} 
    \caption{
    \textbf{Synthetic data collection.} One frame of synthetic data is collected by merging multi-view depth maps into a single-point cloud. Global coordinate noise and per-point noise are applied to simulate realistic conditions.
    This image shows an example of a point cloud created from three depth images.
    }
    \label{fig_s1}
  \end{minipage}

  \vspace{0.3cm} % Adjust vertical space between the figures

  \begin{minipage}{\columnwidth}
    \centering
    \includegraphics[width=\columnwidth]{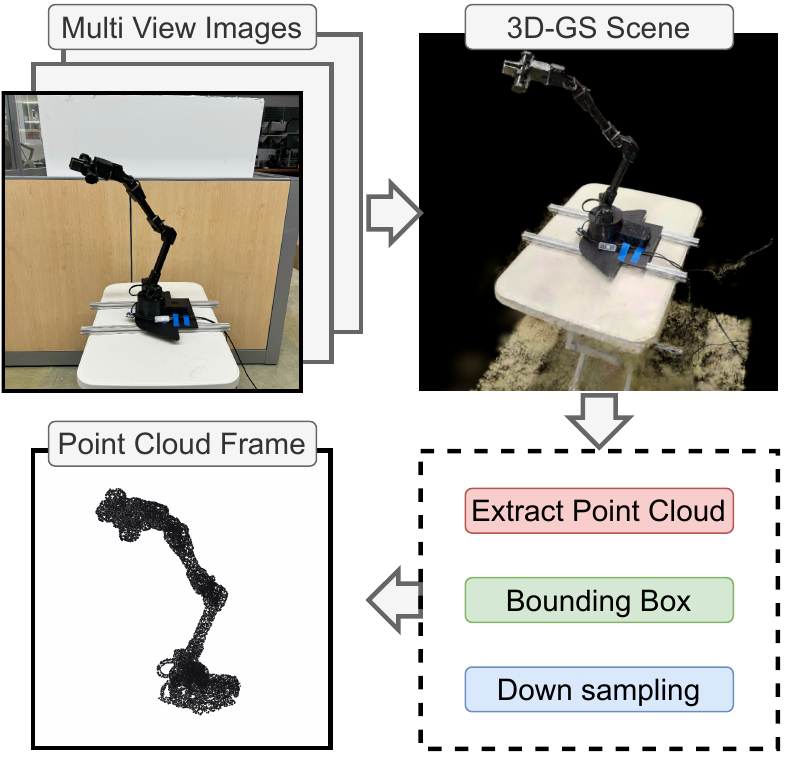}
    \caption{
    \textbf{Real-world data collection.} For each motion step, we capture a video of the robot arm, reconstruct the 3D scene using a 3D Gaussian splatting application \cite{scaniverse, kerbl3Dgaussians}, and extract the point cloud. A bounding box removes background points, and down-sampling standardizes the number of points.
    }
    \label{fig_s2}
  \end{minipage}
\end{figure}

\begin{figure*}[!t]
  \centering
  \includegraphics[width=\textwidth]{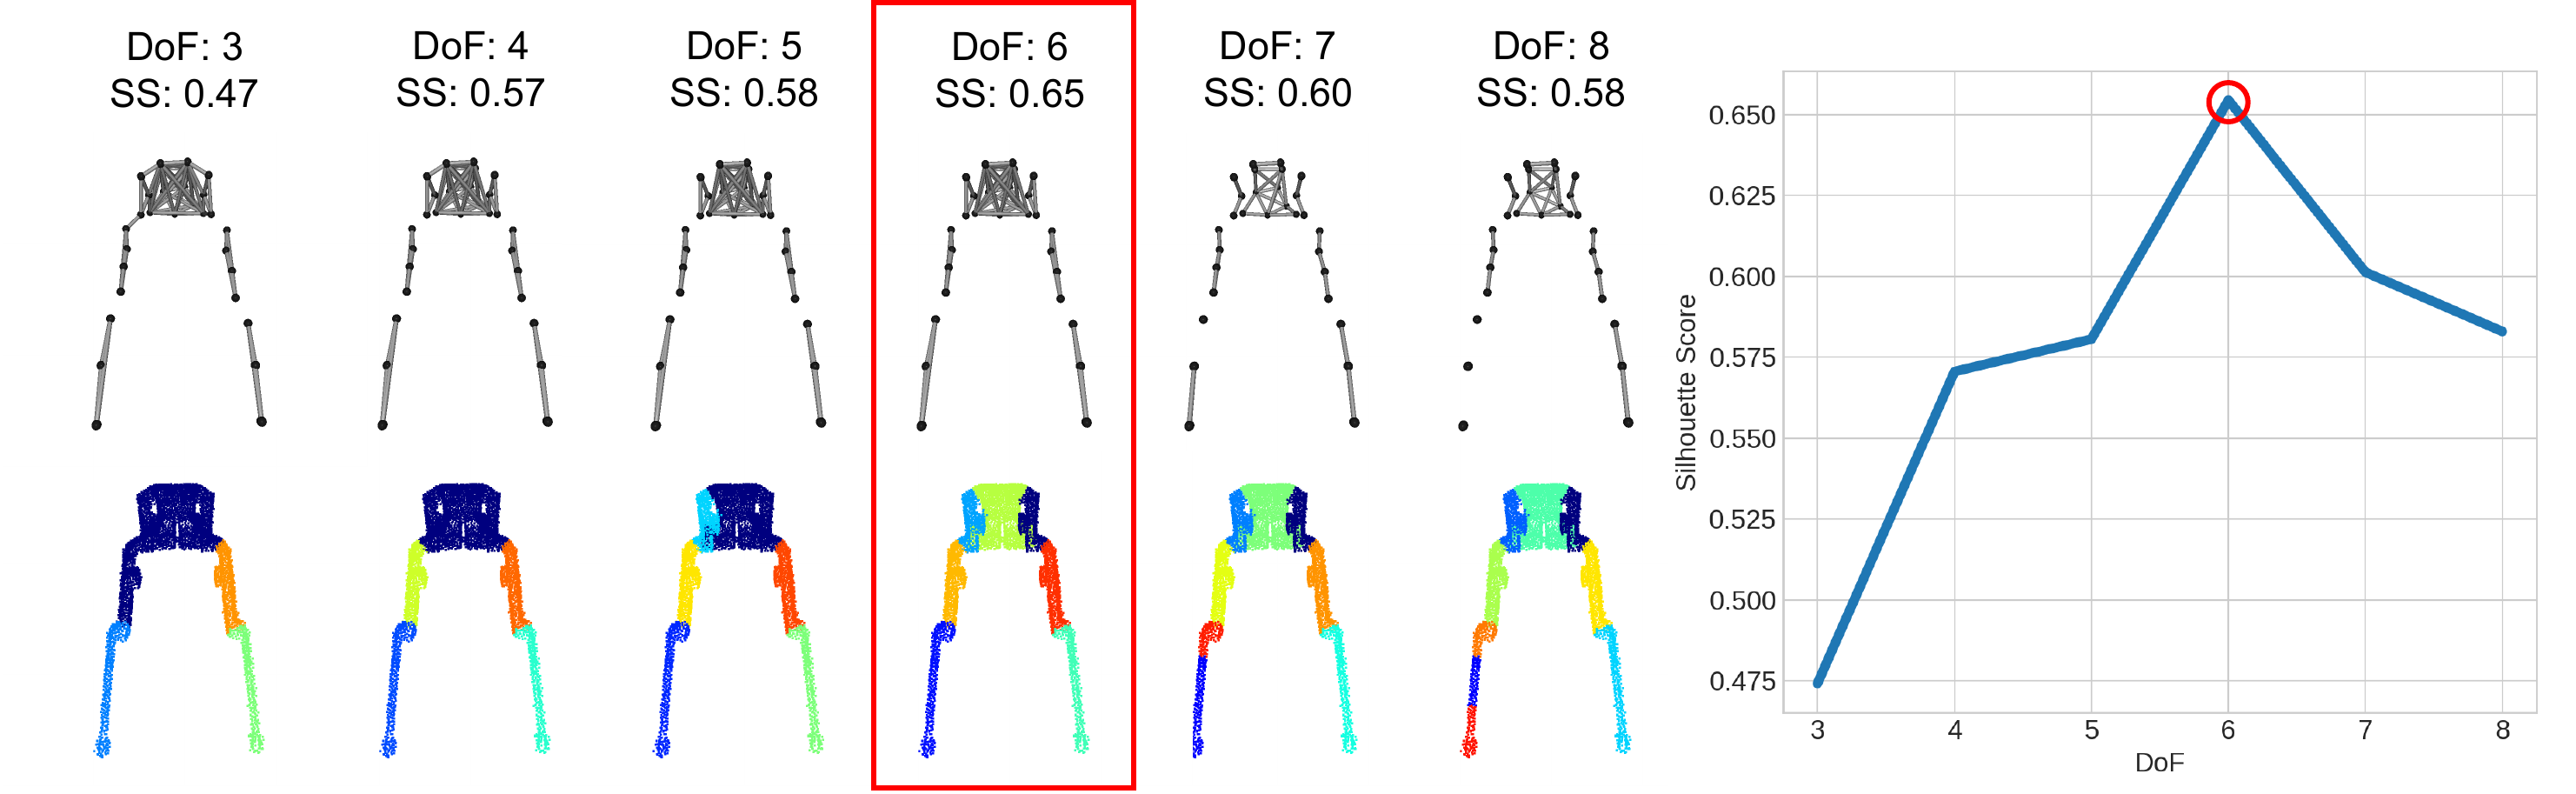}
  \caption{
  \textbf{Silhouette Score Method.} An example of using the Silhouette Score method to identify distinct moving parts and predict the degrees of freedom (DoF) for the Bolt bipedal robot, with a peak score at DoF = 6. This indicates that segmenting the point clusters into seven parts provides the optimal grouping.
    }
    \label{fig_s3}
\end{figure*}

\subsection{Real-world Data}
As shown in Figure \ref{fig_s2}, we conducted real-world experiments using 10 consecutive point cloud scans of a WX200 robot arm, controlling all five motors. The robot was operated through a ROS2 interface, following a randomly sampled motor angle sequence.

Point cloud data was collected using an iPhone camera and the iOS scanning application Scanverse \cite{scaniverse}. A bounding box was applied to isolate the robot arm's point cloud from the environment. Despite the real scan data containing misaligned coordinates across time-steps and significant surface noise, our method directly processes the raw point cloud data, achieving accurate segmentation and URDF generation.

\section{Method Details}
\label{sec:method_details}
\subsection{Silhouette Score Method for Part Segmentation}
Figure \ref{fig_s3} illustrates an example of using the Silhouette Score \cite{rousseeuw1987silhouettes} method to identify the number of links. With DoF ranging from 3 to 8, the averaged Silhouette Score peaks at DoF = 6, which is the correct prediction for the Bolt robot. 
Given the number of groups for the segmentation algorithm, the Silhouette Score and Coefficient are calculated as equation \ref{eq_s1} and equation \ref{eq_s2}.
\begin{equation}
  \label{eq_s1}
  \boldsymbol{SS}(i) = \frac{b(i) - a(i)}{\max(a(i), b(i))}
\end{equation}
\begin{equation}
  \label{eq_s2}
  \boldsymbol{SC} = \max_k \frac{1}{S} \sum_i \boldsymbol{SS}(i)
\end{equation}
In Equation \ref{eq_s1}, $\boldsymbol{SS}(i)$ denotes the Silhouette Score of the $i$-th node, which, in our case, is a point cluster. The term $a(i)$ represents the average distance of the $i$-th node to all other nodes within the same group, while $b(i)$ represents the average distance to nodes in the nearest group. The distance is calculated using Equation \ref{eq3}. $\boldsymbol{SC}(i)$ is the Silhouette Coefficient, which depends on the number of groups, $k$. $S$ represents the total number of nodes. To determine the optimal number of groups for segmentation, we maximize the average Silhouette Score over all groups.

\subsection{Topology Inference}
% In this section
% As shown in algorithm \ref{alg:alg2}, topology inference is divided into three main stages to construct the body topology graph $\boldsymbol{\mathcal{G}}$.
% First, it constructs a list of link dictionaries by identifying connected 
% components from the segmentation graph $G_{seg}$. Each link is initialized 
% with its unique ID, parent link ID, and its connected link IDs, based on the Minimum Spanning Tree $G_{mst}$. 
% Second, the algorithm derives the kinematic tree by iteratively traversing 
% the constructed links. Starting with the root link, it identifies child 
% links by excluding the parent link and updates the hierarchical relationships.
% In the final stage, the body topology graph $\boldsymbol{\mathcal{G}} = (I, E)$ is constructed, where $I$ is the set of link IDs, and $E$ consists of directed edges representing parent-child relationships.
As shown in Algorithm \ref{alg:alg2}, topology inference is divided into three main stages to construct the body topology graph $\boldsymbol{\mathcal{G}}$. In the first stage, the algorithm identifies connected components from the segmentation graph $G_{seg}$, grouping clusters into link components $\{I_c\}$. For each component, it determines its neighboring components using the Minimum Spanning Tree $G_{mst}$, identifying clusters that are directly connected, and therefore the corresponding groups of direct connection. A dictionary is created for each link, containing a unique identifier (\textit{Id}), a parent link initially set to \textit{None}, and a list of connected link IDs. These dictionaries are stored in the list \textit{Links} for further processing. In the second stage, the kinematic tree structure is derived by iteratively traversing the links. Starting with the root link, which is chosen as the first link sorted by ascending center movements, child links are identified by excluding their parent link from the list of connected links. The algorithm updates the parent-child relationships and adds the child links to the next layer for processing. This process continues layer by layer until all links are processed. In the final stage, the body topology graph $\boldsymbol{\mathcal{G}} = (I, E)$ is constructed, where $I$ is the set of link IDs, and $E$ consists of directed edges representing parent-child relationships. 
% This structured approach ensures a clear and systematic inference of the body topology based on the segmentation and spanning tree inputs.

% As shown in Algorithm \ref{alg:alg2}, topology inference consists of three stages to construct the body topology graph $\boldsymbol{\mathcal{G}}$. First, the algorithm identifies connected components from the segmentation graph $G_{seg}$, grouping clusters into link components ${I_c}$. It then determines neighboring components using the Minimum Spanning Tree $G_{mst}$, identifying directly connected clusters and their groups. For each link, a dictionary is created containing a unique identifier (\textit{Id}), a parent link initially set to \textit{None}, and a list of connected link IDs, which are stored in \textit{Links} for further processing. Second, the kinematic tree is derived by traversing the links iteratively. Starting with the root link (the first link sorted by ascending center movements), child links are identified by excluding their parent link from the list of connected links. Parent-child relationships are updated, and child links are added to the next layer for further processing. This step continues until all links are processed. Finally, the body topology graph $\boldsymbol{\mathcal{G}} = (I, E)$ is built, where $I$ is the set of link IDs, and $E$ represents directed edges for parent-child relationships.

\begin{algorithm}[htbp]
\caption{Topology Inference}\label{alg:alg2}
\begin{algorithmic}
  \STATE \textbf{Input}: Segmentation $\boldsymbol{\mathcal{G}_{seg}}$, MST $\boldsymbol{\mathcal{G}_{mst}}$ \par
  \STATE \textbf{Output}: Body Topology $\boldsymbol{\mathcal{G}}$ \par
  \STATE \textbf{Initialize}: $Links \leftarrow \text{EmptyList}$ \par
  \STATE \textbf{Initialize}: $\mathcal{I}_c$ = \text{connected\_components}($\boldsymbol{\mathcal{G}_{seg}}$) \par
  \STATE where $\mathcal{I}_c$ is a list of cluster indices $\{I_c\}$ \par

\texttt{//} 1. Construct a list of link dictionaries\par
\textbf{for} ($I_l$, $\{I_c\}$) \textbf{in} enumerate($\mathcal{I}_c$) \par
\hspace{1em} Find connected clusters \par
\hspace{1em} \textbf{for} $I_c$ \textbf{in} $\{I_c\}$ \par
\hspace{2em} $\{I_{\text{c\_connected}}\} \leftarrow \boldsymbol{\mathcal{G}_{\text{mst}}}.\text{neighbors}(I_c)$ \par
\hspace{1em} \textbf{end for} \par
\hspace{1em} Find connected links $\{I_{\text{l\_connected}}\}$ with $\{I_{\text{c\_connected}}\}$ \par
\hspace{1em} Build dictionary: Link = \{\par
\hspace{4em} Id: $I_l$; \par
\hspace{4em} parent: \text{None}; \par
\hspace{4em} connected\_links: $\{I_{\text{l\_connected}}\}$\}\par
\hspace{1em} $Links.\text{append(Link)}$\par
\textbf{end for} \par
Sort $links$ by center movements in ascending order\par
\texttt{//} 2. Derive the kinematic tree\par
\STATE \textbf{Initialize:} $current\_layer$ = [$links$[0]] \texttt{//} root\par
  \REPEAT
    \STATE Initialize $next\_layer \gets \emptyset$, $child\_set \gets \emptyset$
    \FOR{$\text{Link}_{current}$ \textbf{in} $current\_layer$}
        \IF{$\text{Link}_{current}$ has parent}
            \STATE $child \gets \text{connected\_links excluding parent}$
        \ELSE
            \STATE $child \gets \text{connected\_links}$
        \ENDIF
        \FOR {$\text{Link}_{child}$  \textbf{in} $child$}
            \STATE Update $\text{Link}_{child}$.parent $\gets \text{Link}_{current}.\text{Id}$
            \STATE Add $\text{Link}_{child}$ to $next\_layer$
        \ENDFOR
        \STATE Update $child\_set \gets child\_set \cup child$
    \ENDFOR
    \STATE Update $current\_layer \gets next\_layer$
  \UNTIL{$child\_set = \emptyset$}\par
\texttt{//} 3. Build $\boldsymbol{\mathcal{G}}$ from $Links$\par
\STATE $\boldsymbol{\mathcal{G}} = (I, E)$ \par
where $I = \{ \text{Link.Id} \}$, $ E = \{ (\text{Link}.parent, \text{Link.Id}) \}$
\end{algorithmic}
\label{alg2}
\end{algorithm}

\subsection{Model Architecture}

Figure \ref{fig_s4} shows the architecture of the registration model. We use a shared neural network to predict incremental updates to the position and rotation of each point cluster. The input dimensions align with the pose representation of the point clusters. A sinusoidal positional encoder enhances the network's ability to capture spatial relationships and patterns\cite{tancik2020fourfeat}. The model includes a fully connected encoder and separate decoders for rotation and position. The network's output is added to the input coordinates to learn incremental updates directly. We use PyTorch \cite{torch} to implement the model and optimization is performed using the Adam optimizer\cite{kingma2014adam}.

The same model architecture is applied to both the Step Model and the Anchor Model, with learning rates of 0.0001 and 0.00005, respectively. The training loss is calculated using the L1 Chamfer distance between the transformed point cloud and the ground truth. An early stopping mechanism halts optimization if the point cloud error does not decrease after a set number of steps, ensuring efficient training.

\begin{figure}[!t]
  \centering
  \includegraphics[width=\columnwidth]{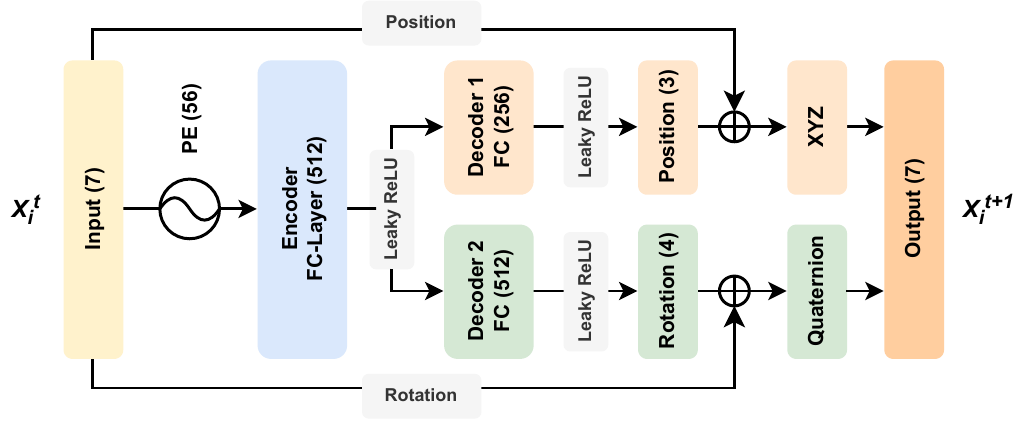}
  \caption{
  \textbf{Registration Model Architecture.} We developed a lightweight neural network for point cluster registration, employing the same model architecture for both the Step Model and Anchor Model.
    }
    \label{fig_s4}
\end{figure}

\begin{figure}[!t]
  \centering
  \includegraphics[width=\columnwidth]{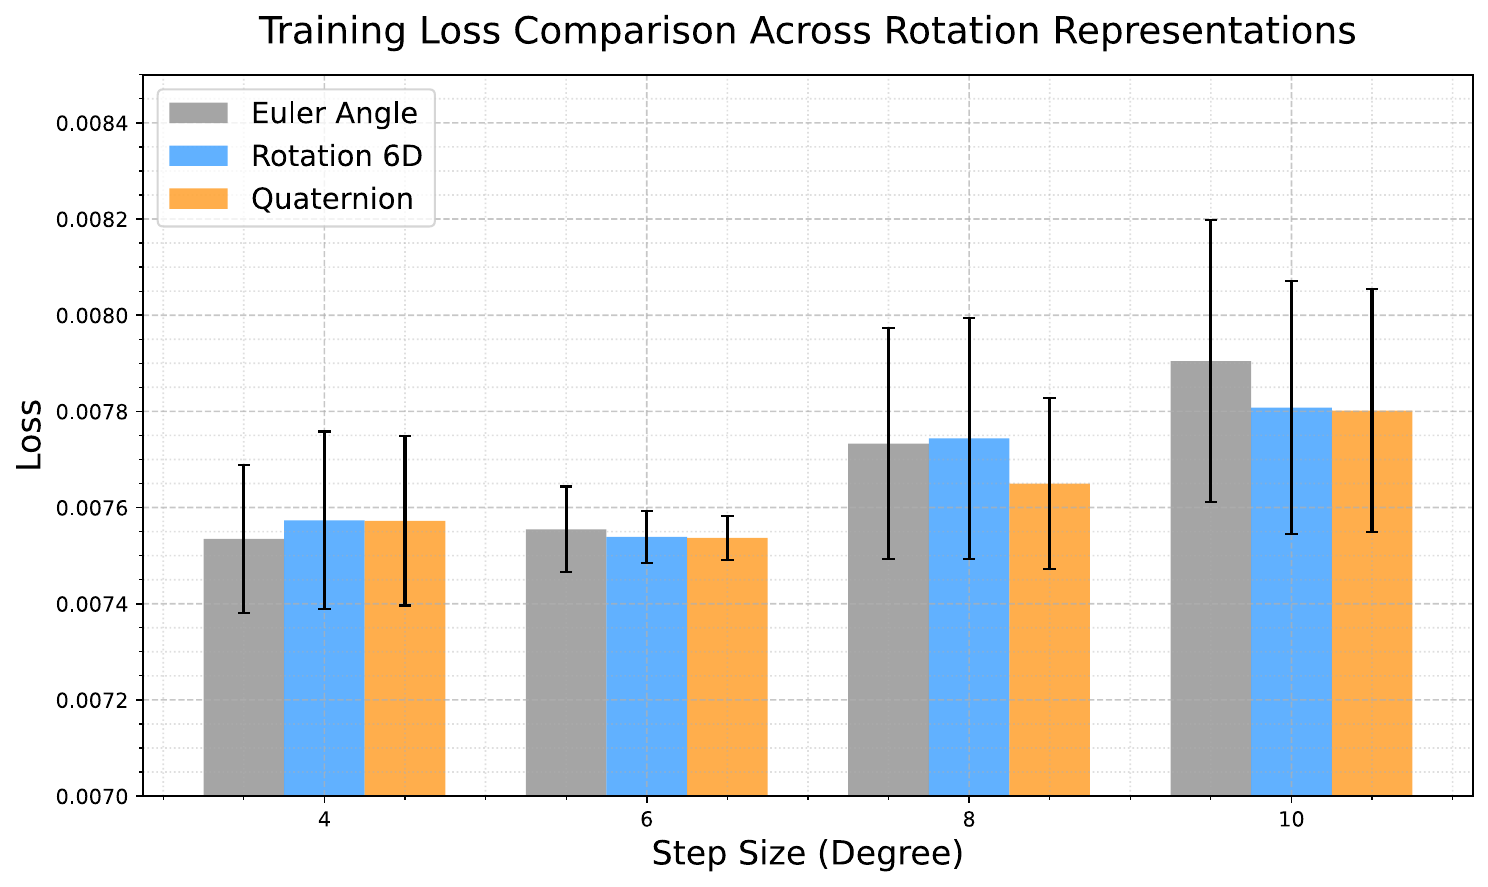} 
  \caption{
  \textbf{Training Loss Comparison of Rotation Representations Across Step Sizes.} 
    }
    \label{fig_s5}
\end{figure}

\begin{figure}[!t]
  \centering
  \includegraphics[width=\columnwidth]{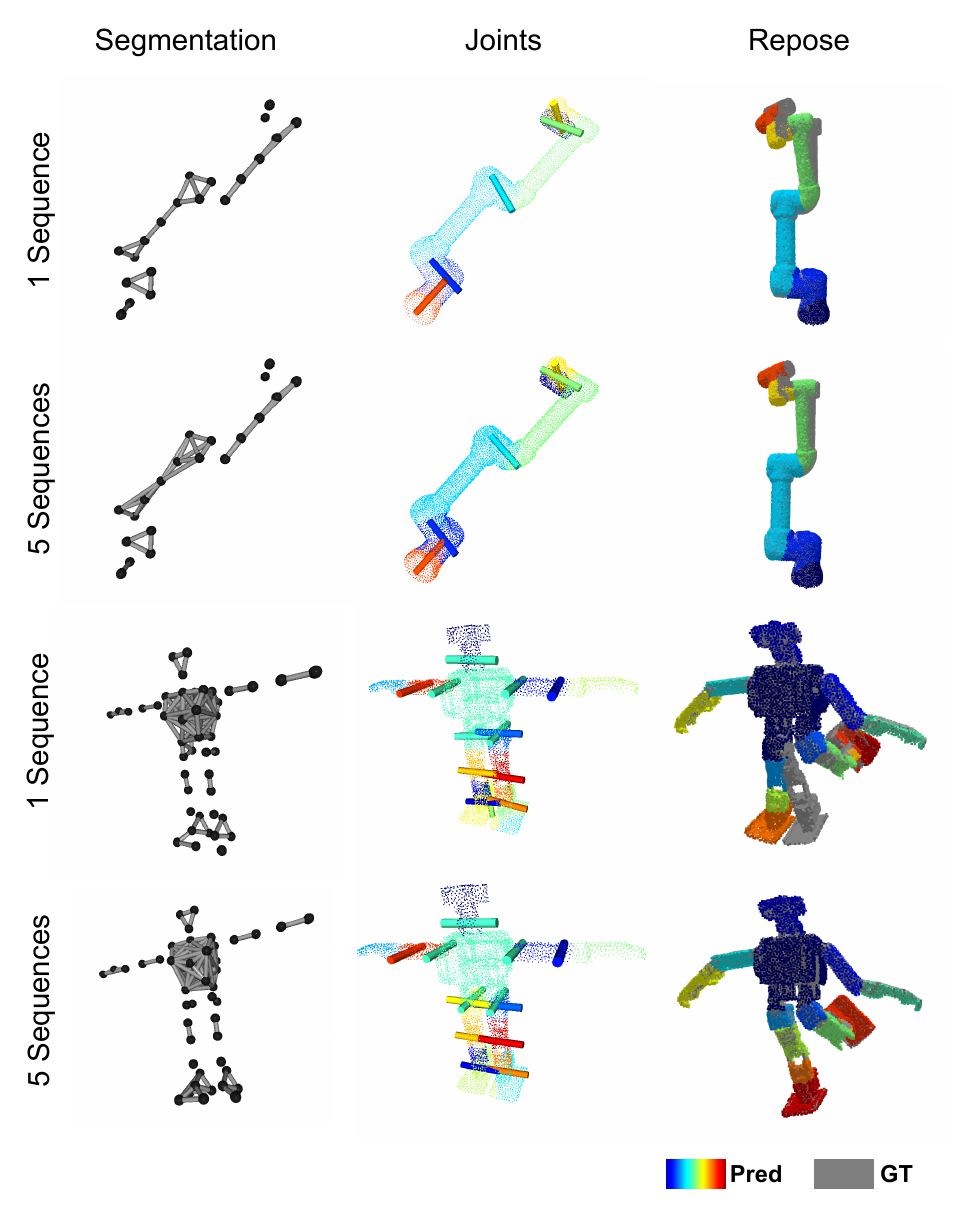} 
  \caption{
  \textbf{Qualitative Comparison on Different Number of Input Sequences.}
    }
    \label{fig_s6}
\end{figure}

\begin{figure}[!t]
  \centering
  \includegraphics[width=\columnwidth]{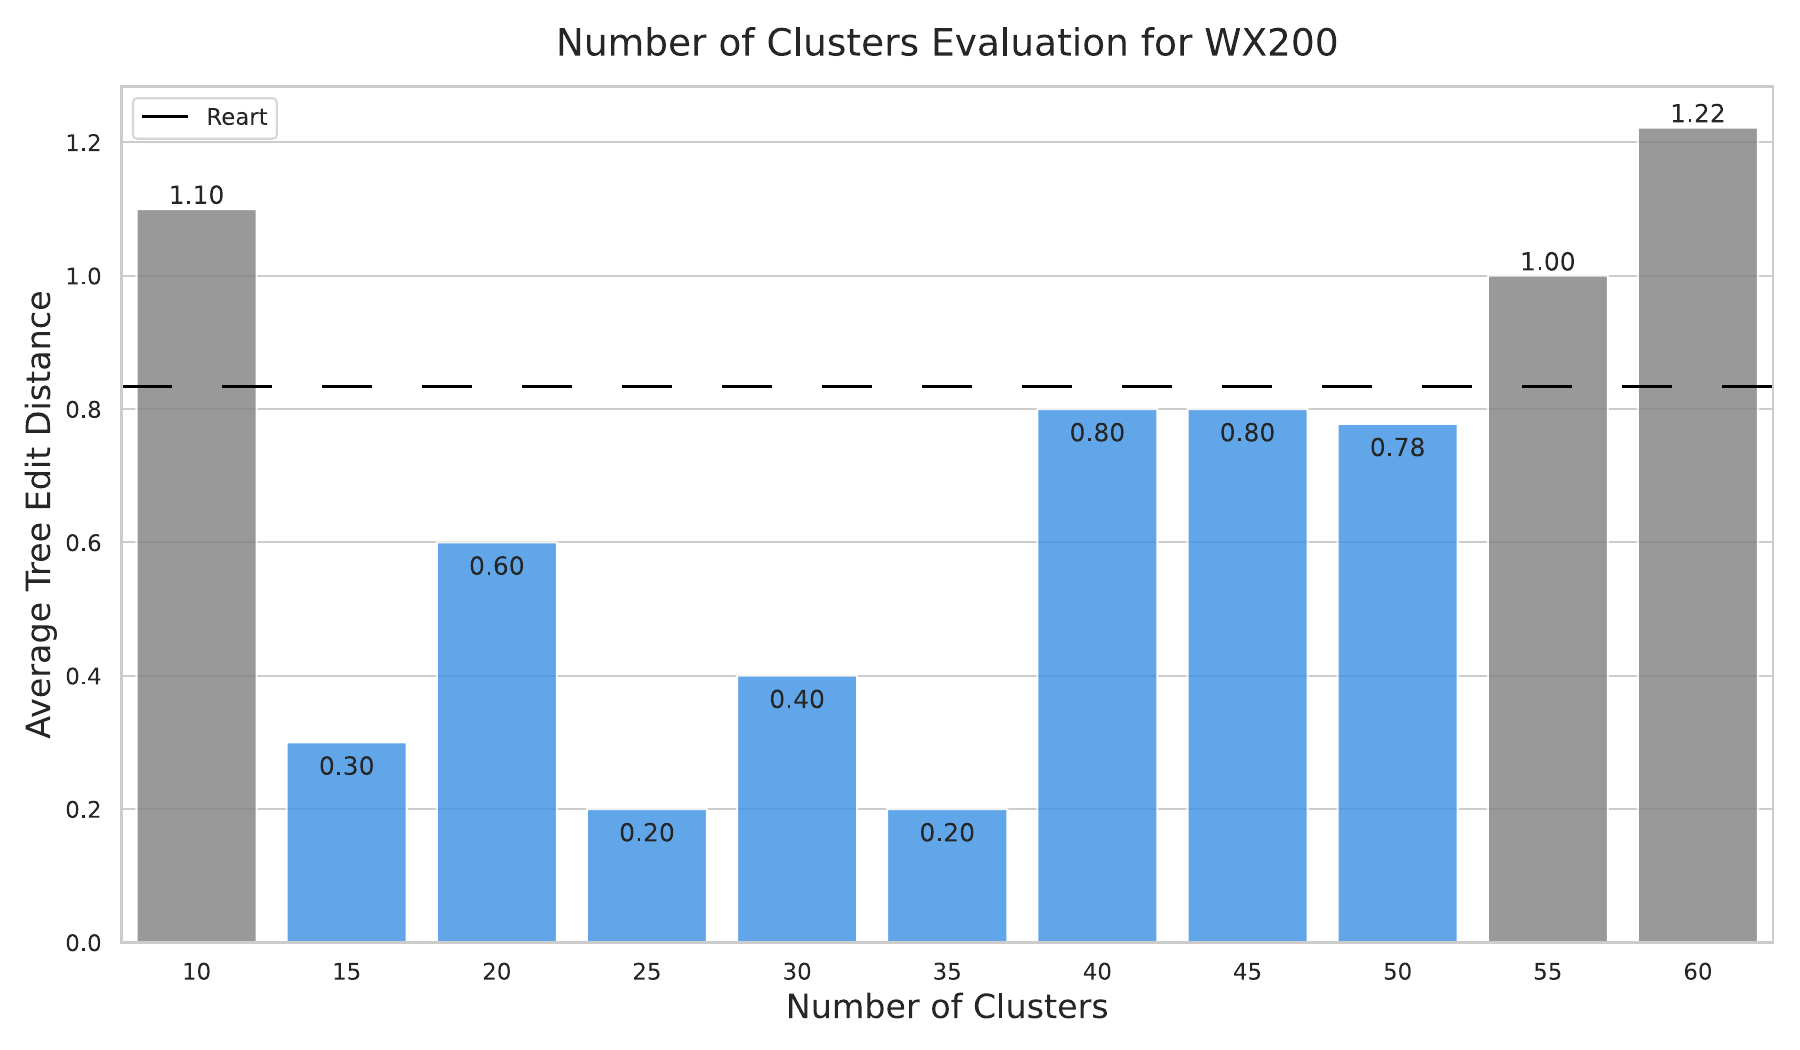}
  \includegraphics[width=\columnwidth]{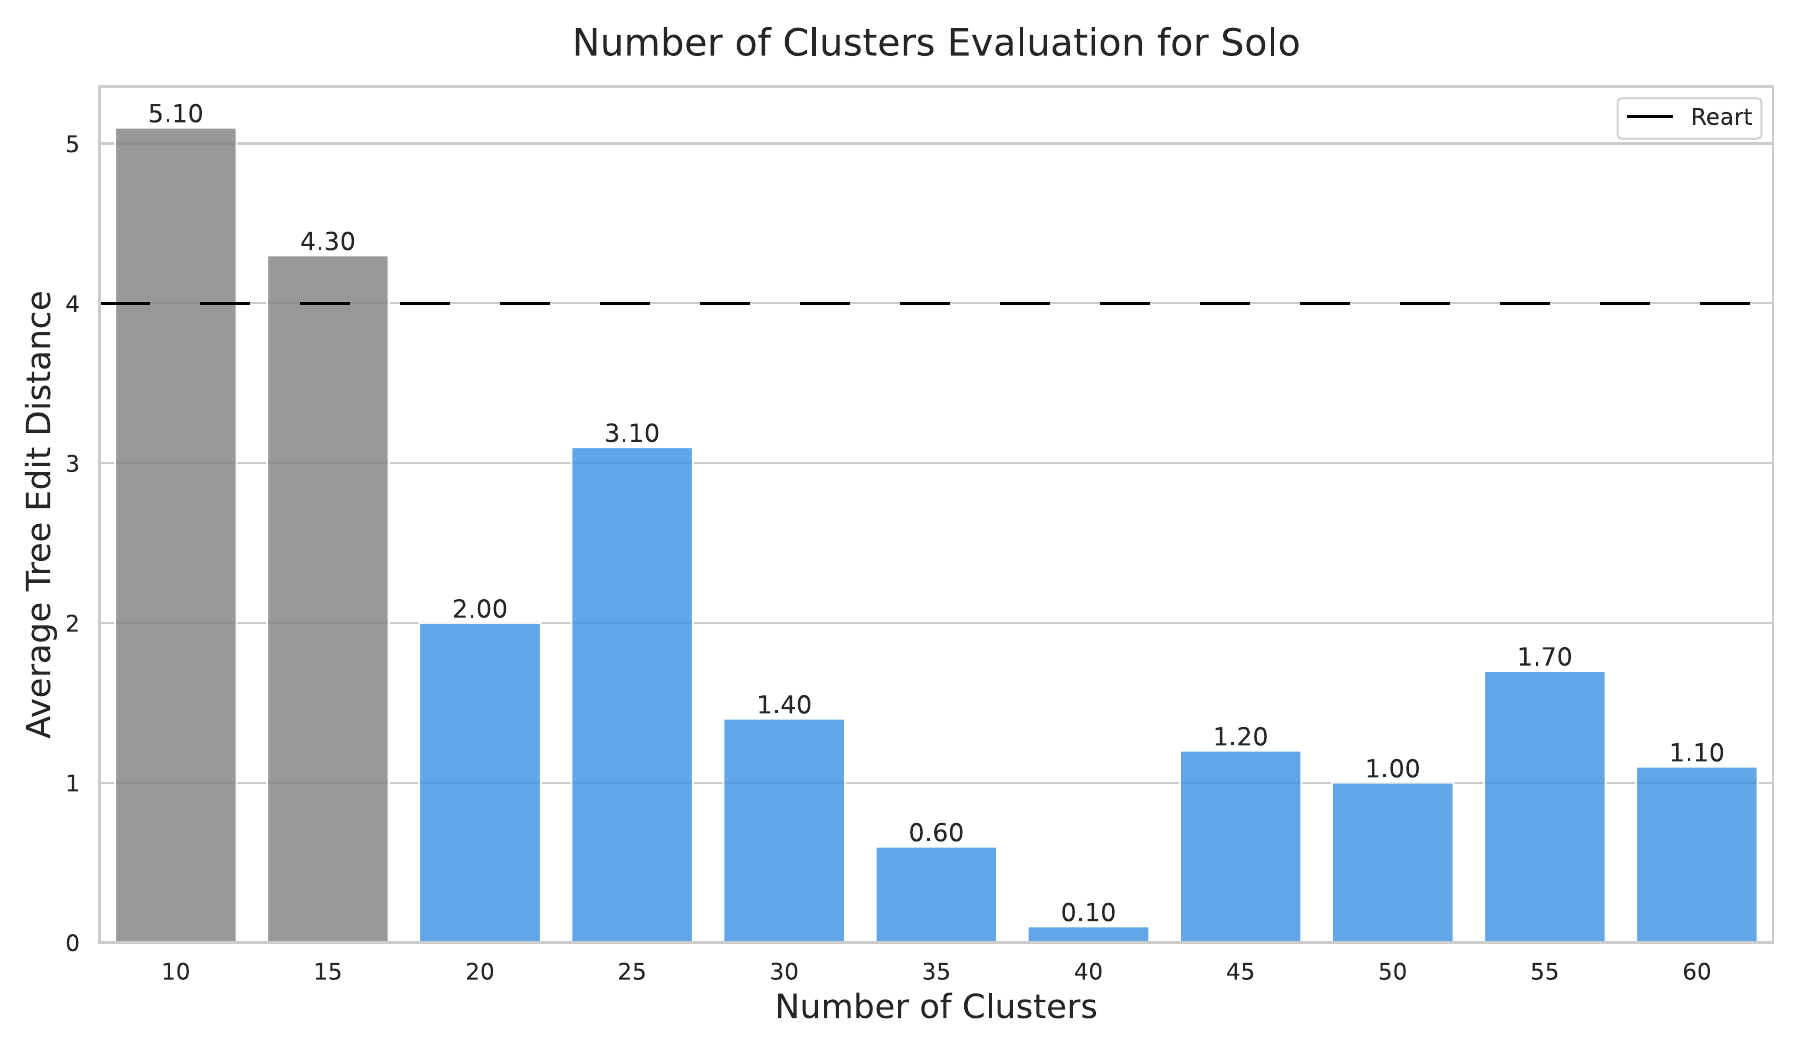} 
  \includegraphics[width=\columnwidth]{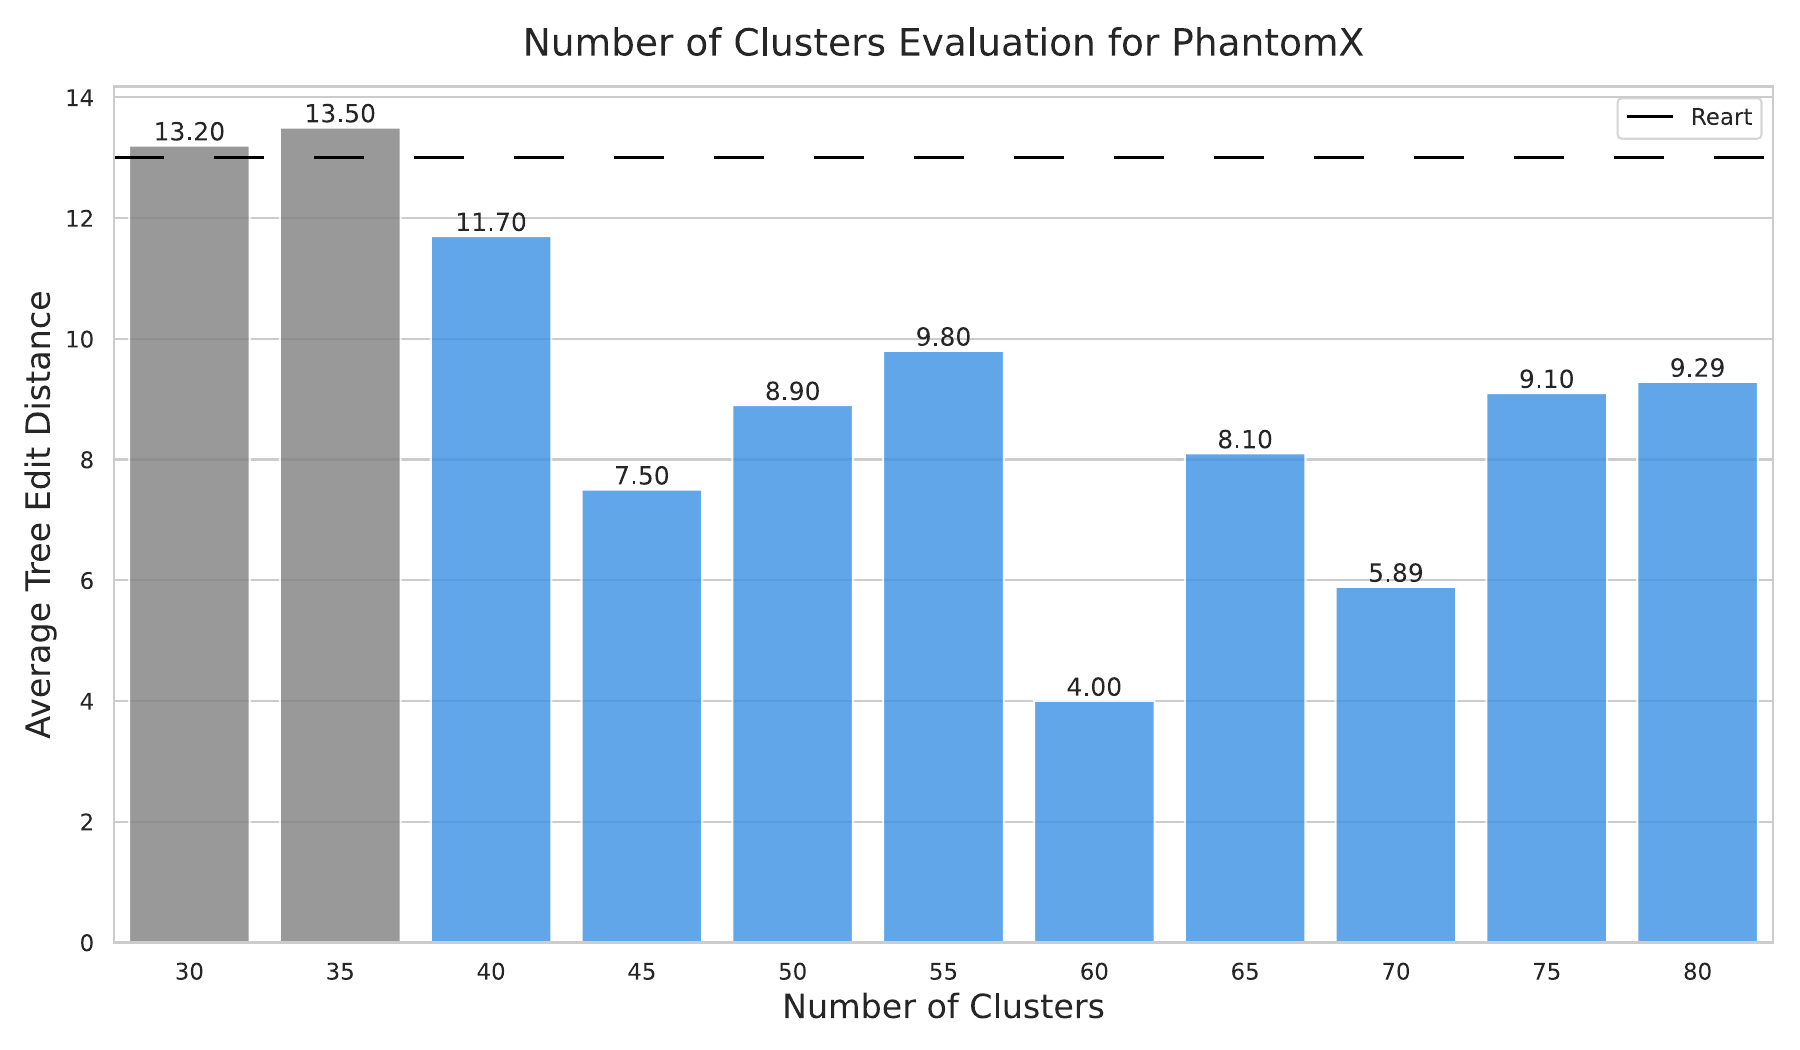} 
  
  \caption{
  \textbf{Impact of Cluster Number on Tree Edit Distance.}
    }
    \label{fig_s7}
\end{figure}

\begin{figure*}[!t]
  \centering
  \includegraphics[width=\textwidth]{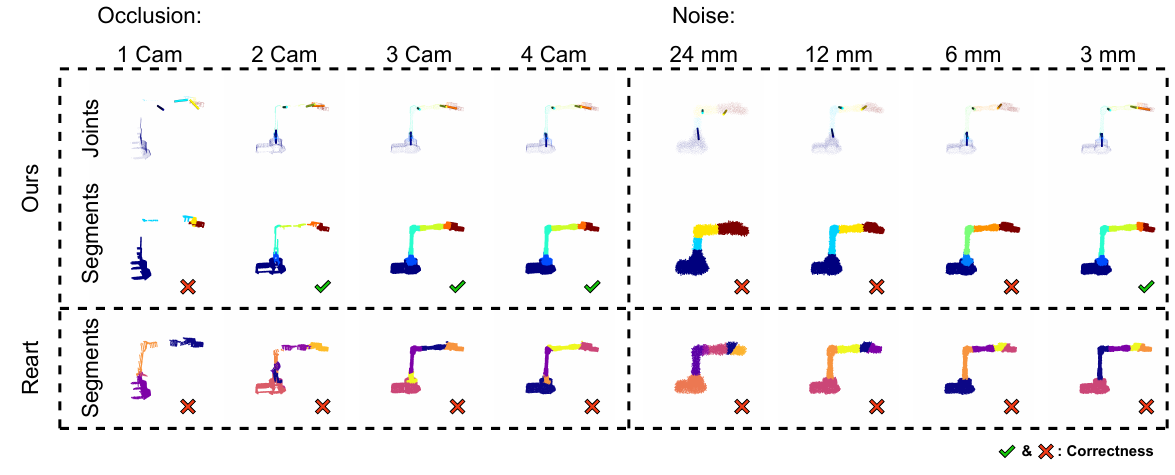}
  \caption{
  \textbf{Impact of completeness and noise of input point cloud.}
    }
    \label{fig_sr}
\end{figure*}

\subsection{Rotation Representation}
To efficiently and robustly learn the rotation of clusters To optimize the learning of inter-frame cluster rotations in our registration model, we investigate the efficacy of three rotation representations: Euler Angles, Quaternions, and 6D Rotation representations \cite{zhou2019continuity}. We conduct extensive experiments across ten diverse sequences, comparing these representations regarding their training stability and convergence properties. As shown in \ref{fig_s5}, both Quaternions and 6D Rotation representations demonstrate superior robustness as the angular step size increases from 4° to 10°. The empirical results suggest that these continuous representations maintain consistent performance even under larger rotational variations, while Euler Angles show increased instability at higher angles. This aligns with previous findings regarding the advantages of continuous rotation representations in deep learning frameworks. Based on these results, our implementation supports both Quaternion and 6D Rotation representations, with Quaternion as the default configuration.
\begin{figure*}[!t]
  \centering
  \includegraphics[width=\textwidth]{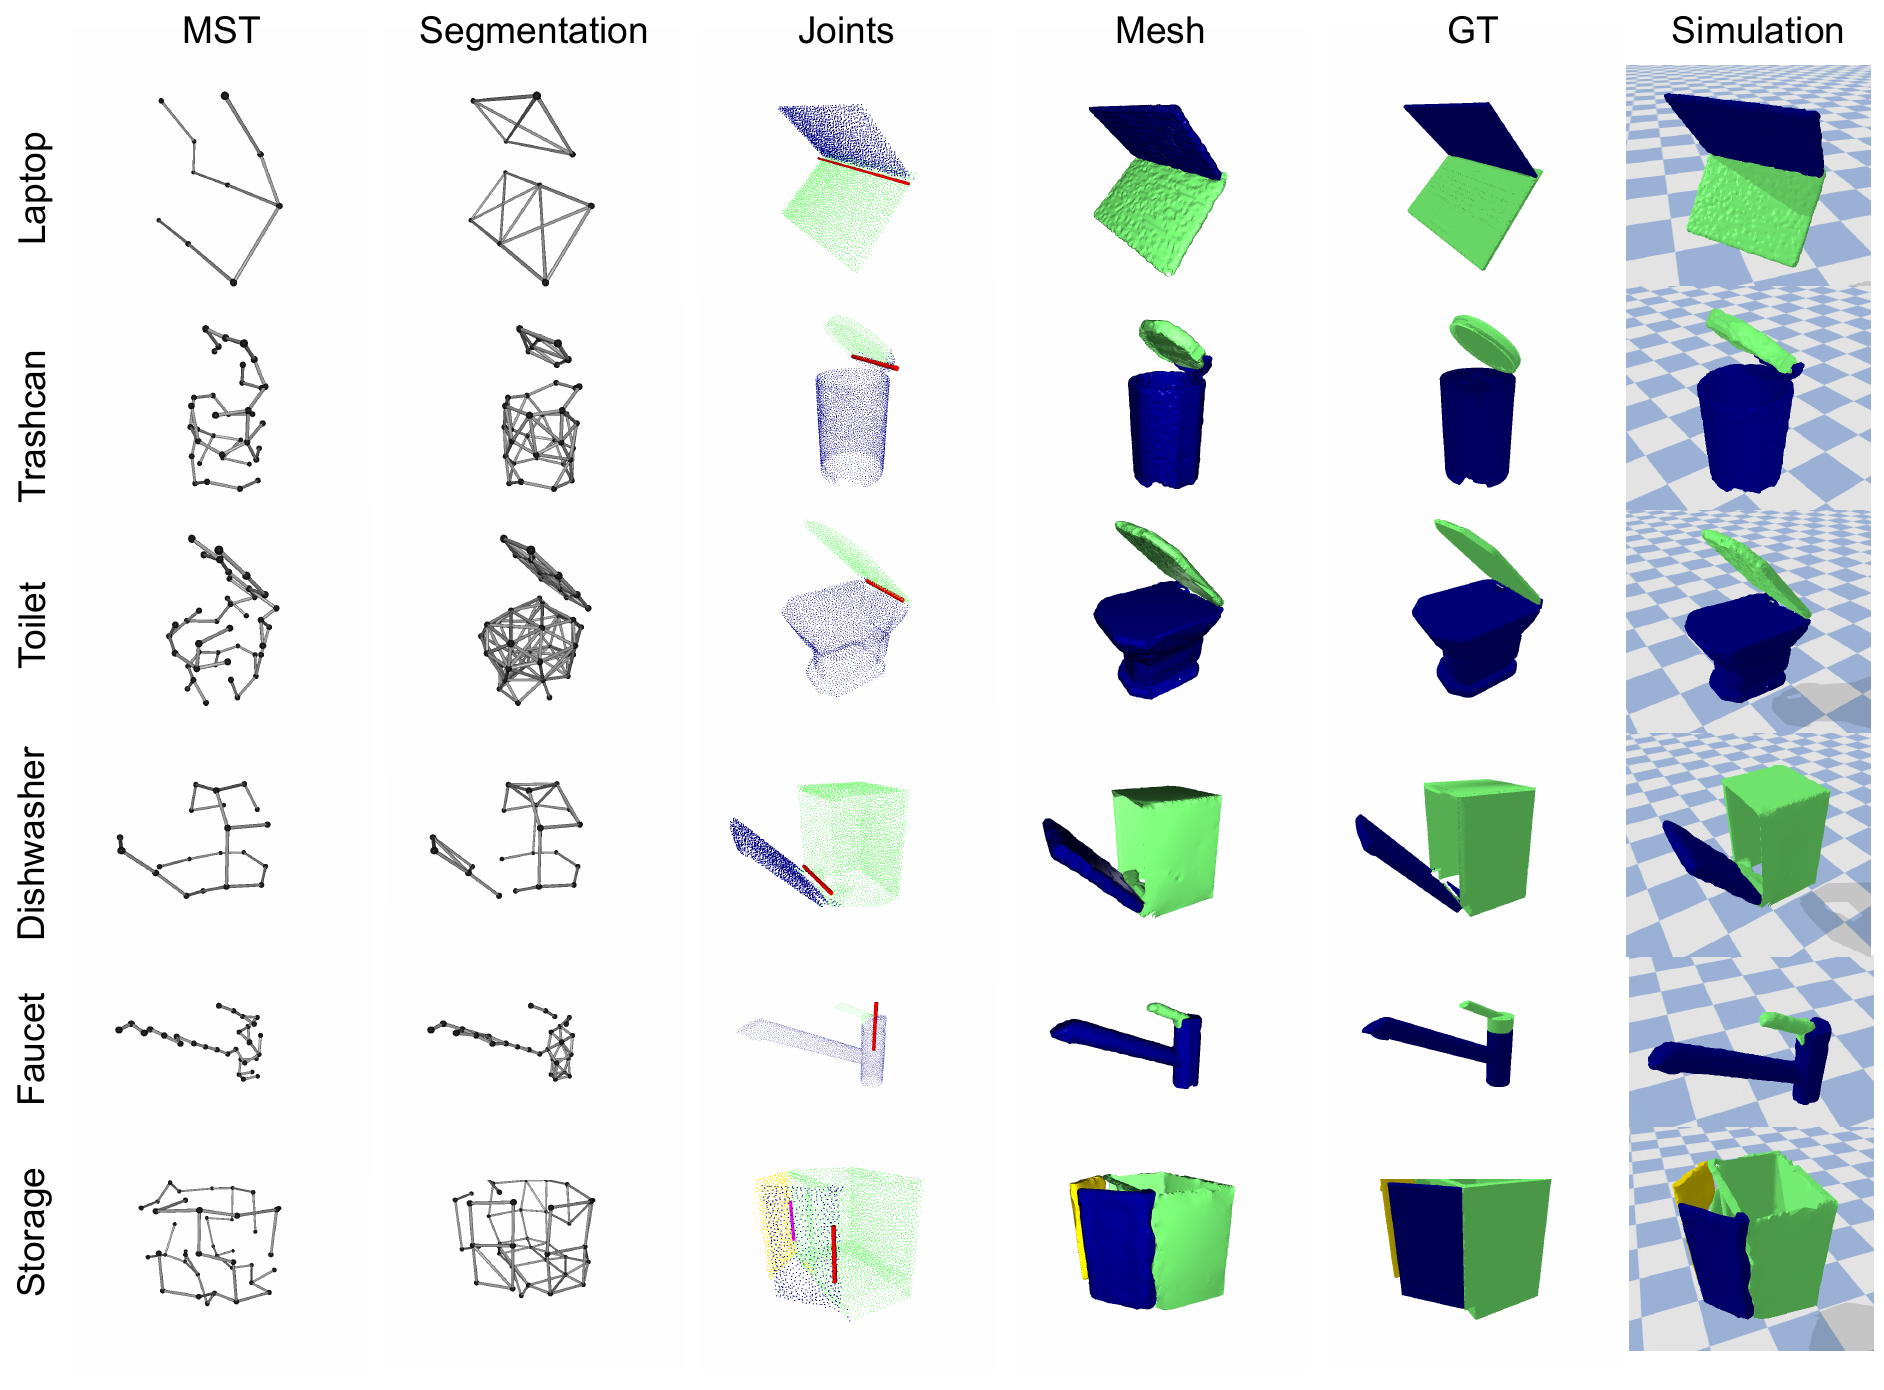} 
  \caption{
  \textbf{Qualitative Results on \textit{PartNet-Mobility} \cite{Mo_2019_CVPR} Dataset.} 
    }
    \label{fig_s8}
\end{figure*}
\begin{figure*}[!t]
  \centering
  \includegraphics[width=\textwidth]{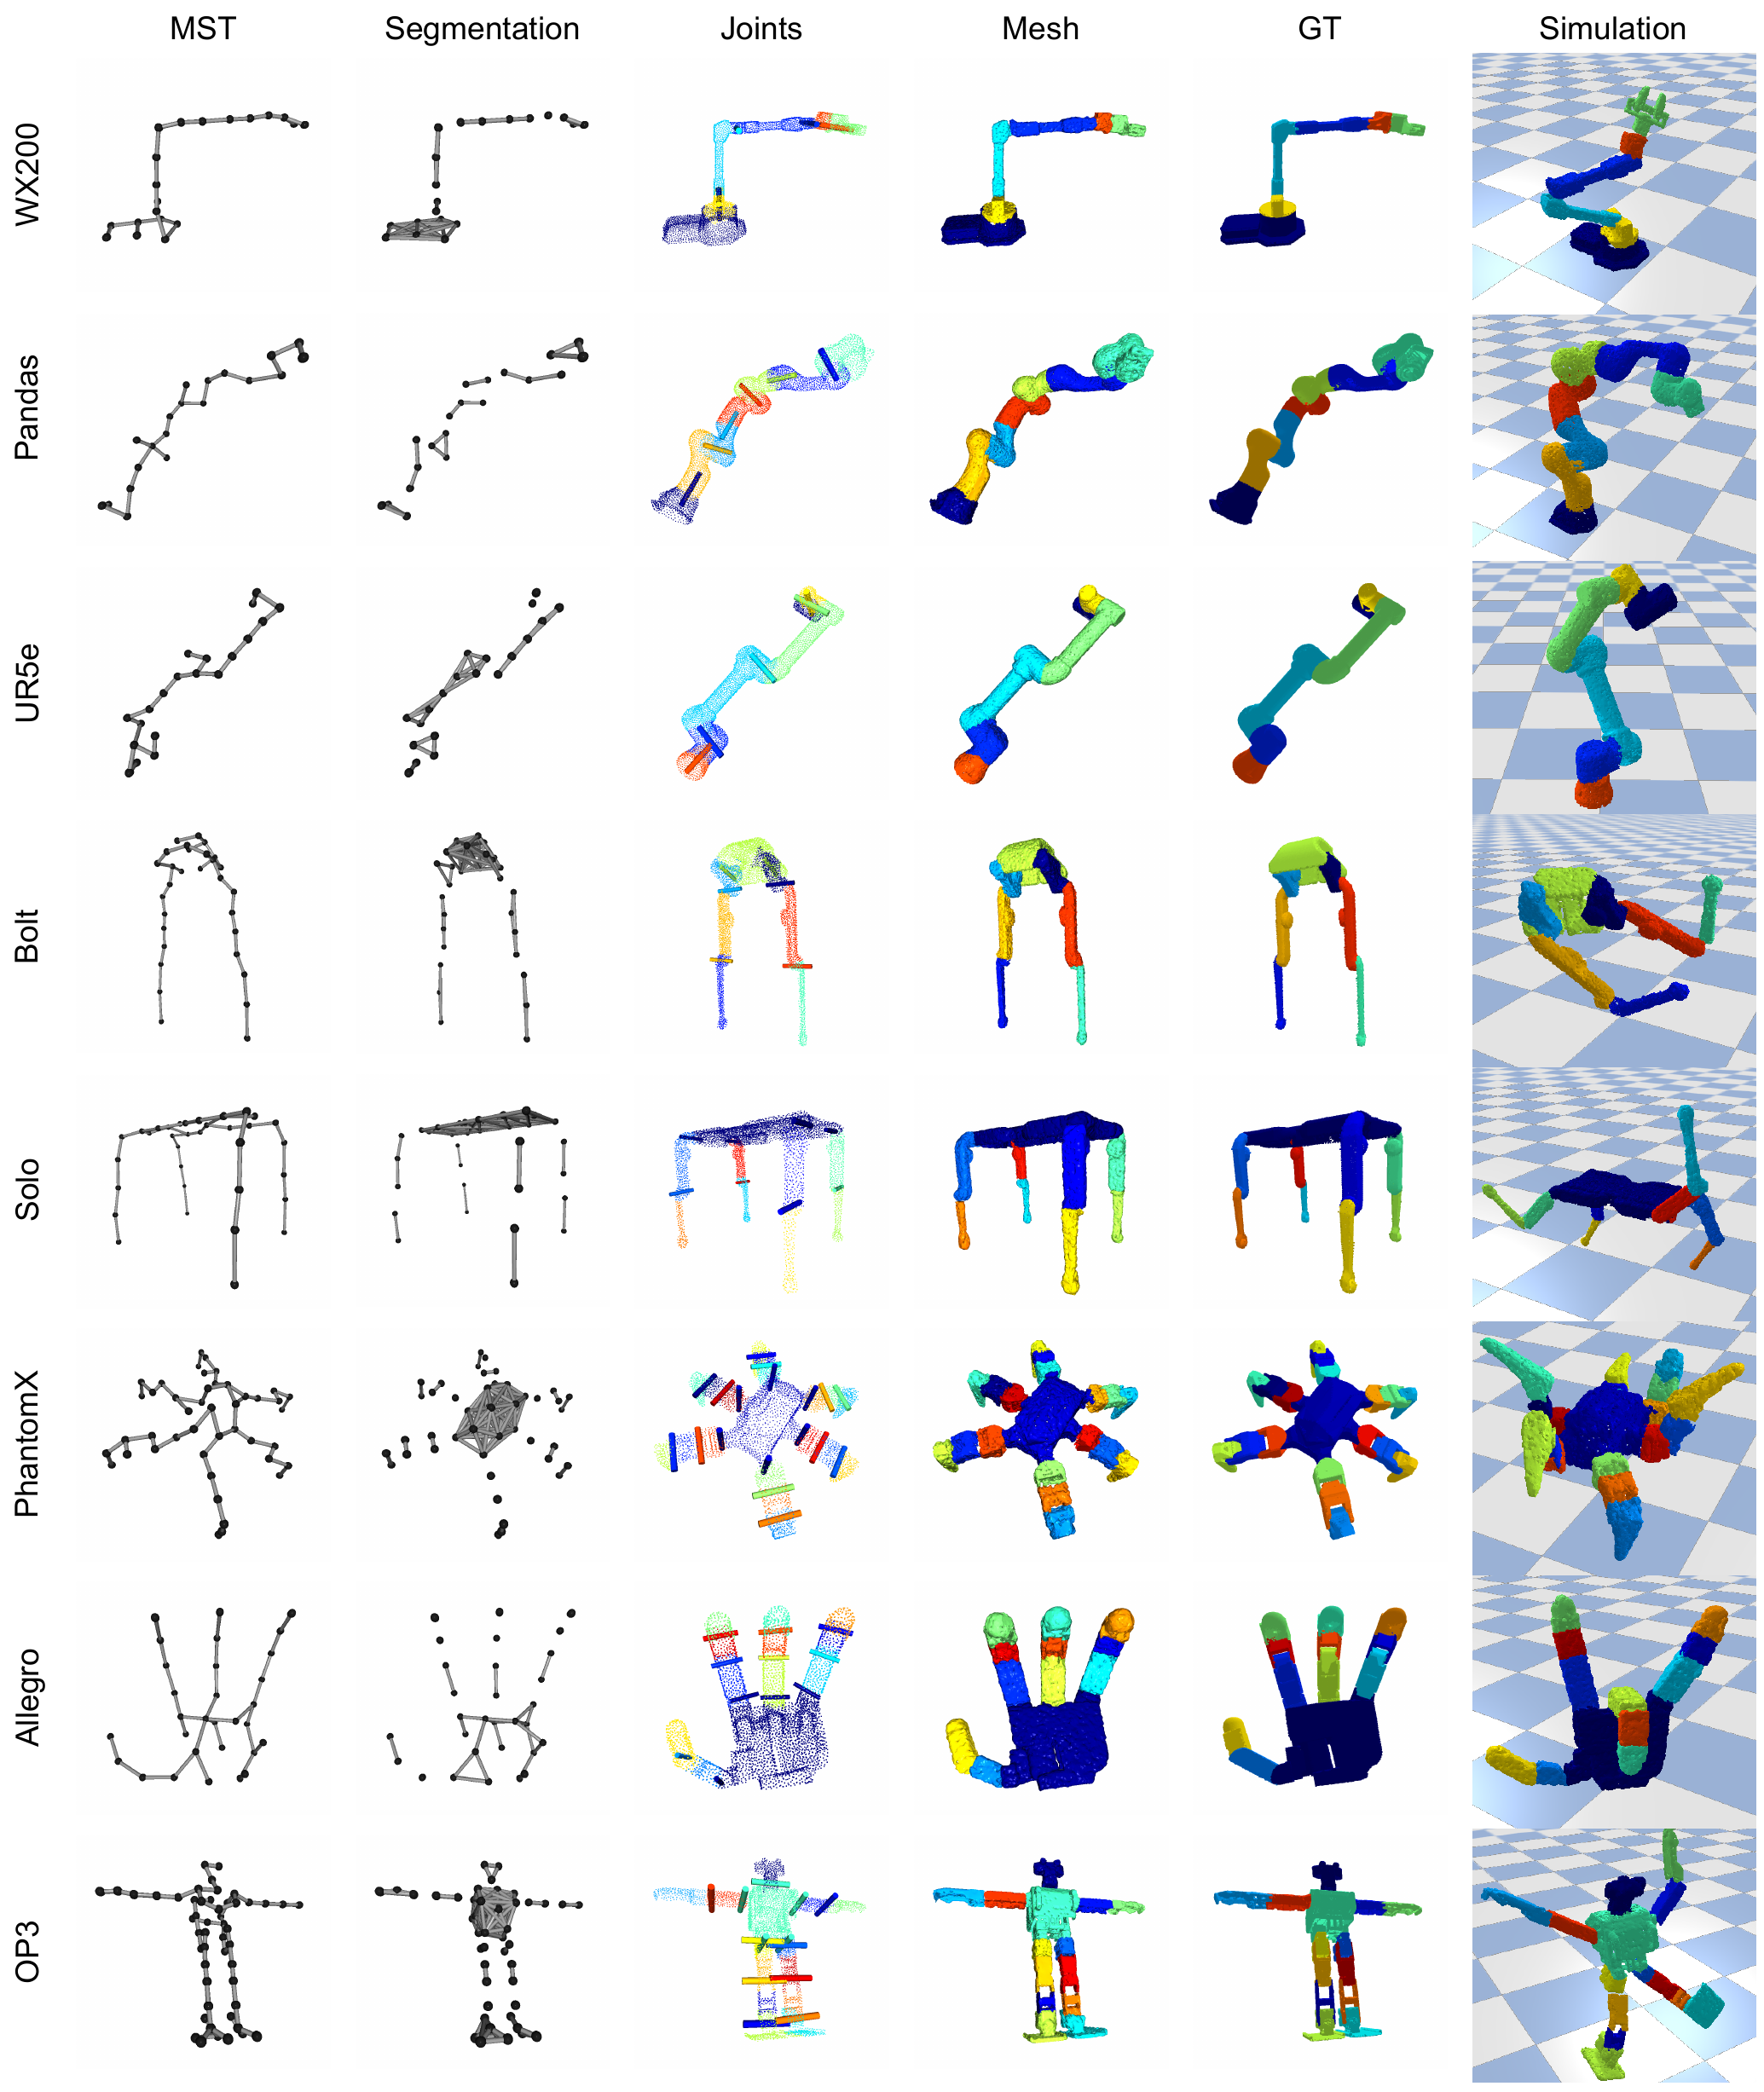} 
  \caption{
  \textbf{Quantative Results on AutoURDF Dataset.} 
    }
    \label{fig_s9}
\end{figure*}

\section{Additional Results}
\label{sec:additional_exp}
\subsection{Experiment on Number of Input Sequences}
The Multi-Sequence Merging Experiment presented in our main text compares the performance of our method using a single sequence of point cloud frames against five sequences of point cloud frames. The results indicate that Our method achieves improved performance in 7 out of 8 robots for both repose evaluation and joint distance evaluation while demonstrating improvements across all robots for joint angle evaluation.
Additionally, Figure \ref{fig_s6} provides a qualitative comparison. With data from five sequences, our method generates segmentations with higher distinction, creating more edges within the correct group of point clusters, as exemplified in the UR5 robot. Furthermore, it achieves higher accuracy in joint estimation and reposed point cloud generation. 

With the starting motor configurations aligned across different sequences, our method merges multiple sequences by registering them to the same set of point clusters and averaging the resulting motion correlation matrices. We perform the repose comparison by repeating the synthetic point cloud collection process (Figure \ref{fig_s1}) using a new set of random motor configurations applied to both the predicted and ground-truth URDFs.

\subsection{Experiment on Number of Clusters}

To investigate the sensitivity of our method to the quality and refinement level of initial clusters, we conduct extensive experiments across robots with varying structural complexity. We evaluate each robot configuration across eleven different cluster quantities, comparing against the \textit{Reart} baseline \cite{liu2023building}. As shown in \ref{fig_s7}, we observe that while optimal performance occurs at specific cluster number ranges, our method consistently outperforms the baseline (indicated by blue bars) across a wide range of parameter settings, demonstrating the method's stability across different robot architectures.

Evaluation across three robot configurations (WX200, Solo, PhantomX) with varying structural complexity. Blue bars indicate performance superior to \textit{Reart} \cite{liu2023building}, shown as the dashed line.

\subsection{Experiment on Occlusion and Noise}

To evaluate the robustness of our algorithm in real-world conditions, we tested it under varying levels of \textbf{noise and occlusion} by adding Gaussian noise and limiting the number of camera views (Fig. \ref{fig_sr}). The results show that our method outperforms \textit{Reart} \cite{liu2023building} in highly noisy and occluded scenarios, in terms of moving parts segmentation.

\subsection{Experiment on \textbf{\textit{PartNet-Mobility}} Dataset}
We evaluate our AutoURDF framework on six common household articulated objects from the \textit{PartNet-Mobility} dataset \cite{Mo_2019_CVPR}, each featuring one or two degrees of freedom: laptop, trashcan, toilet, dishwasher, faucet, and storage cabinet. As shown in \ref{fig_s8}, we initialize each object in an open configuration to facilitate distinct part clustering. To enhance the initial segmentation of planar components, we incorporate k-means clustering with normal information from the point cloud. The framework demonstrates robust performance in both segmentation and joint parameter estimation for objects with predominantly planar structures. While the cylindrical geometry of the faucet presents challenges for precise segmentation, the framework still maintains accurate joint axis prediction, highlighting its robustness to partial segmentation errors.

% 
% To split the supplementary pages from the main paper, you can use \href{https://support.apple.com/en-ca/guide/preview/prvw11793/mac#:~:text=Delete%20a%20page%20from%20a,or%20choose%20Edit%20%3E%20Delete).}{Preview (on macOS)}, \href{https://www.adobe.com/acrobat/how-to/delete-pages-from-pdf.html#:~:text=Choose%20%E2%80%9CTools%E2%80%9D%20%3E%20%E2%80%9COrganize,or%20pages%20from%20the%20file.}{Adobe Acrobat} (on all OSs), as well as \href{https://superuser.com/questions/517986/is-it-possible-to-delete-some-pages-of-a-pdf-document}{command line tools}.
